# Supplementary material for: Annual field-scale maps of tall and short crops at the global scale using GEDI and Sentinel-2
Source: arXiv:2212.09681 source file (2022-12-19)
Supplement: Supplementary file 1 [file appendix.tex]

\appendix
\section*{Appendix}

\clearpage
